# Supplementary material for: Towards Universal & Efficient Model Compression via Exponential Torque Pruning
Source: arXiv:2506.22015 source file (2025-07-03)
Supplement: Supplementary file 1 [file appendix.tex]

% \section{Appendix}

% \section{Grouping strategy}
% \newpage
% \section{Training Setup}
% In this section, we introduce the detailed training setup of both our methods and the compared baselines. Concretely, \lzm{...}
% We formalize our grouping strategies for different layer types in a model-agnostic manner, defining groups based on the structural properties of each layer. Given a neural network with parameters \(\theta\), we partition \(\theta\) into disjoint sets \(\{G_i\}\), where each \(G_i\) represents a grouped parameter subset determined by the layer type:

% \begin{itemize}
%     \item \textbf{Fully Connected (Linear) Layers}: Each neuron \(h_j\) in a layer with weight matrix \(W \in \mathbb{R}^{m \times n}\) is treated as a grouped component, i.e., \(G_j = \{W_{:, j}, b_j\}\).
%     \item \textbf{Convolutional Layers}: Each filter \(F_k \in \mathbb{R}^{c \times h \times w}\) is considered a grouped parameter, such that \(G_k = \{F_k\}\).
%     \item \textbf{Attention Layers}: Each attention head \(A_t\) is treated as a grouped parameter, where \(G_t = \{W_t^Q, W_t^K, W_t^V, W_t^O\}\).
% \end{itemize}

% By defining these layer-specific grouping strategies mathematically, we establish a principled framework that facilitates the application of SORTS across diverse neural network architectures.

\section{Training Setup}

\begin{table}[!h]
\centering
\caption{Training configurations for ETP across all evaluated benchmarks. Standard schedules are used per task to ensure fair comparison with the compared baselines.}
\label{tab:etp_training}
\normalsize
\begin{adjustbox}{width=0.98\textwidth}
\begin{tabular}{@{}p{3.5cm}p{1.2cm}p{1.8cm}p{4.5cm}p{5.5cm}@{}}
\toprule
\textbf{Dataset (Model)} & \textbf{Epochs} & \textbf{Batch Size} & \textbf{LR Scheduler} & \textbf{Optimizer} \\ 
\midrule
CIFAR-10 (ResNet-56)     & 100   & 128 & MultiStepLR (milestones = [60, 80], $\gamma=0.1$) & SGD (lr = 0.001, momentum = 0.9, weight decay = $5\text{e}{-4}$) \\[1ex]
CIFAR-100 (VGG-19)       & 100   & 128 & MultiStepLR (milestones = [60, 80], $\gamma=0.1$) & SGD (lr = 0.001, momentum = 0.9, weight decay = $5\text{e}{-4}$) \\[1ex]
ImageNet-1k (ResNet-50)  & 90    & 256 & StepLR (step size = 30, $\gamma=0.1$)             & SGD (lr = 0.1, momentum = 0.9, weight decay = $1\text{e}{-4}$) \\[1ex]
MRPC (BERT)              & 10    & 32  & Linear decay with 10\% warm-up                   & AdamW (lr = $2\text{e}{-5}$, weight decay = 0.01) \\[1ex]
SST-2 (BERT)             & 10    & 32  & Linear decay with 10\% warm-up                   & AdamW (lr = $2\text{e}{-5}$, weight decay = 0.01) \\[1ex]
MRPC (RoBERTa)           & 10    & 32  & Linear decay with 10\% warm-up                   & AdamW (lr = $2\text{e}{-5}$, weight decay = 0.01) \\[1ex]
SST-2 (RoBERTa)          & 10    & 32  & Linear decay with 10\% warm-up                   & AdamW (lr = $2\text{e}{-5}$, weight decay = 0.01) \\[1ex]
PPI (GAT)                & 1000  & 1   & CosineAnnealingLR ($T_{\max}=1000$)              & Adam (lr = 0.005, weight decay = $5\text{e}{-4}$) \\[1ex]
ETTh1 (Informer)         & 6     & 32  & CosineAnnealingLR ($T_{\max}=6$)                 & Adam (lr = $5\text{e}{-4}$, weight decay = $1\text{e}{-4}$) \\
\bottomrule
\end{tabular}
\end{adjustbox}
\end{table}
In this section, we detail the training configuration of our proposed method and the baseline approaches. 
First, for ETP, we use the following strategy for all tasks to select the $\lambda$ and $\beta$ for our loss function.
The regularization coefficient $\beta$ is selected via grid search over the range $\{10^{-6},\ 5\times10^{-6},\ 10^{-5},\ 5\times10^{-5},\ 10^{-4},\ 5\times10^{-4},\ 10^{-3}\}$. The optimal value of $\beta$ varies depending on the model architecture and the desired pruning aggressiveness. Higher compression rates are obtained by increasing $\beta$ accordingly. For the exponential base $\lambda$, we defined it as a function of the number of grouped parameters in a layer $l$: $\lambda_{l} = \exp\left(\frac{5}{|\mathcal{G}_l|}\right)$, 
where $|\mathcal{G}_l|$ denotes the total number of parameter groups (e.g., convolutional filter, attention head, \etc). The detailed training setup of ETP for all the evaluated benchmarks is illustrated in \Cref{tab:etp_training}. We strictly follow the experimental setup of the compared baselines according to their provided implementations for fair comparison.
% The parameters of DepGraph are selected the same as the reproduce section of the DepGraph repository as found at this link (\href{DepGraph}{https://github.com/VainF/Torch-Pruning}). For GReg and Torque, we attempt to reproduce the results, however due to improper documentation of the hyperparameters used in the loss function, we are unable to reproduce it for all the tasks hence we select the best of the reproduce results and the results represented in the paper.

\section{Additional experiments on L2-norm learning process}
We further present additional results of the L2-norm analysis during training process on Informer (ETTh1) and BERT (MRPC) as a supplementary of RQ1. The detailed results are shown in \Cref{fig:l2_append}. It is obvious that the results are consistent with that of RQ1. For example, for Informer trained and evaluated on ETTh1, ETP manages to optimally prune both investigated modules ($m^l_{4}, m^l_{12}$) as ETP deems them redundant for effective inference (\ie~L2-norm equals to 0 ($||m^l_{4}||=0.0,\ ||m^l_{12}||=0.0$)), while the ones regularized by the vanilla Torque remains a high L2-norm for these modules (\ie~$||m^l_{4}||=0.99,\ ||m^l_{12}||=2.44$). The extensive L2-norm analysis during the training process validate that the exponential force application scheme can indeed help ETP achieve a much sparser neural network architecture, and therefore achieve a much higher compression rate with lower performance drop.

\begin{figure}
    \centering
    \includegraphics[width=0.9\linewidth]{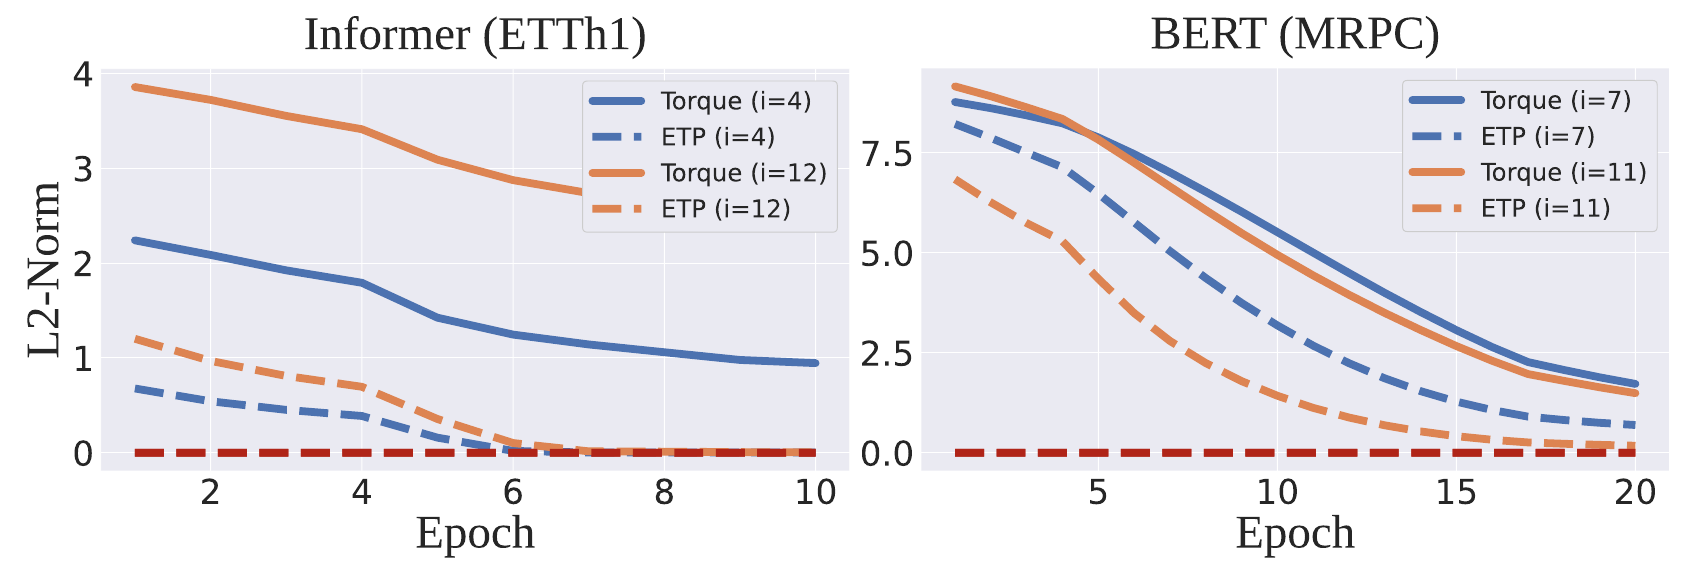}
    \caption{Additional results on the l2-norm analysis during the training process.}
    \label{fig:l2_append}
\end{figure}
